# Supplementary material for: Rethinking Class-Balanced Methods for Long-Tailed Visual Recognition from a Domain Adaptation Perspective
Source: arXiv:2003.10780 source file (2020-03-24)
Supplement: Supplementary file 1 [file supp_separate.tex]

% \documentclass[10pt,twocolumn,letterpaper]{article}

% \usepackage{cvpr}
% \usepackage{times}
% \usepackage{epsfig}
% \usepackage{graphicx}
% \usepackage{amsmath}
% \usepackage{amssymb}
% \usepackage{subfigure}
% \usepackage{algorithm,algpseudocode,bm}
% \usepackage{xcolor}



% % Include other packages here, before hyperref.

% % If you comment hyperref and then uncomment it, you should delete
% % egpaper.aux before re-running latex.  (Or just hit 'q' on the first latex
% % run, let it finish, and you should be clear).
% \usepackage[pagebackref=true,breaklinks=true,letterpaper=true,colorlinks,citecolor=blue,linkcolor=blue,bookmarks=false]{hyperref}

% \def\thesection{\Alph{section}}

% \newcommand{\BG}[1]{\textcolor{blue}{BG: #1}}
% \newcommand\matt[1]{{\color{purple}[matt: #1]}}
% \newcommand\cut[1]{}

% \cvprfinalcopy % *** Uncomment this line for the final submission

% \def\cvprPaperID{8760} % *** Enter the CVPR Paper ID here
% \def\httilde{\mbox{\tt\raisebox{-.5ex}{\symbol{126}}}}

% % Pages are numbered in submission mode, and unnumbered in camera-ready
% \ifcvprfinal\pagestyle{empty}\fi
% \begin{document}

% %%%%%%%%% TITLE
% \title{Rethinking Class-Balanced Methods for Long-Tailed Visual Recognition \\from a Domain Adaptation Perspective \\ \emph{- Supplementary Materials -}}

% \iffalse
% \author{First Author\\
% Institution1\\
% Institution1 address\\
% {\tt\small firstauthor@i1.org}
% % For a paper whose authors are all at the same institution,
% % omit the following lines up until the closing ``}''.
% % Additional authors and addresses can be added with ``\and'',
% % just like the second author.
% % To save space, use either the email address or home page, not both
% \and
% Second Author\\
% Institution2\\
% First line of institution2 address\\
% {\tt\small secondauthor@i2.org}
% }
% \fi

% \maketitle

% \paragraph{\Large Outline}

% \begin{itemize}
% \item{Multiple runs of experiments on CIFAR-LT-10 under different imbalance factors (IFs). (Section~\ref{sec:multiple}).}
% \item{Detailed comparison of various methods on large-scale long-tailed datasets (Section~\ref{sec:study}).}
% \end{itemize}


% \section{Multiple runs on CIFAR-LT-10} \label{sec:multiple}
% In this experiment, we further validate our approach by running each setting 5 times with different random seeds. Table~\ref{tab:multipleruns} shows the mean top-1 errors (\%) and the standard deviations under the imbalance factor of 200, 100, and 50. We can see that the mean error rates are consistent with the results provided in Table 2 of the main paper.


% \begin{table*}
% \centering
% \caption {\label{tab:multipleruns} Multiple runs of our approach by using the cross-entropy loss on CIFAR-LT-10. The results are top-1 errors\% on the test sets. }
% \vspace{5pt}

% %\resizebox{0.5\textwidth}{!}

% \begin{tabular}{l|c|l|l}
% \hline

% \hline

% \hline
% Imbalance factor & 200 & \multicolumn{1}{c|}{100} & \multicolumn{1}{c}{50} \\ \hline

% Cross-entropy training & 34.32 & 29.64 & 25.19  \\ \hline

% Class-balanced cross-entropy loss~\cite{CBLoss} & 31.11 & 27.63 & 21.95 \\ \hline


% \begin{tabular}[c]{@{}l@{}}Class-balanced fine-tuning\\ Class-balanced fine-tuning*\end{tabular} & \begin{tabular}[c]{@{}c@{}}33.76\\ 33.92\end{tabular} & \begin{tabular}[c]{@{}l@{}}28.66\\ 28.67\end{tabular} & \begin{tabular}[c]{@{}l@{}}22.56\\ 22.58\end{tabular}  \\ \hline

% \begin{tabular}[c]{@{}l@{}}L2RW~\cite{L2RW}\\ L2RW~\cite{L2RW}*\end{tabular} & \begin{tabular}[c]{@{}c@{}}33.75\\ 33.49\end{tabular} & \begin{tabular}[c]{@{}l@{}}27.77\\ 25.84\end{tabular} & \begin{tabular}[c]{@{}l@{}}23.55\\ 21.07\end{tabular}  \\ \hline


% Meta-weight net~\cite{MWN} & 32.8 & 26.43 & 20.9  \\ \hline


% Ours with cross-entropy loss & \textbf{29.32 $\pm$ 0.23}  & \textbf{23.71 $\pm$ 0.22}  & \textbf{19.45 $\pm$ 0.28} \\ \hline
 
% \end{tabular}

% \end{table*}




% % \begin{table*}
% % \centering
% % \caption {\label{tab:updating both weights} Top-1 errors\% on the test set of CIFAR-LT-10 with an imbalance factor of 200 when update both w$_{y}$ and $\epsilon$.}
% % \vspace{5pt}

% % %\resizebox{0.5\textwidth}{!}

% % \begin{tabular}{l|c|l|l}
% % \hline

% % \hline

% % \hline
% % Imbalance factor & 200 & \multicolumn{1}{c|}{100} & \multicolumn{1}{c}{50} \\ \hline

% % Ours & 29.34 & 23.59 & 19.49  \\ \hline

% % Ours, updating w$_{y}$ and $\epsilon$ & 29.72 & 24.16 & 19.81 \\ \hline

% % \end{tabular}

% % \end{table*}



% \section{Detailed comparison of various methods on large-scale long-tailed datasets} \label{sec:study}
% In this section, we present the top-1 errors (\%) of various methods for ImageNet-LT, Places-LT, and iNaturalist 2018\footnote{While we include the comparison on iNaturalist 2018 due to that most existing related works report results on this dataset, we reiterate that we advocate the use of iNaturalist 2017, instead of 2018, in this and future work due to the extremely small validation set of iNaturalist 2018.}. As the experiment setups of the existing works vary by network initialization, the sampling strategy of mini-batches, losses, trainable layers of a network, etc., it is hard to have a fair comparison by the end results. Hence, besides their top-1 errors, we also report the experiment setups for each method. Tables~\ref{tab:ImageNet-LT},~\ref{tab:Places-LT},~and~\ref{tab:iNat18} show the results of the different methods on ImageNet-LT, Places-LT, and iNaturalist 2018, respectively. Our approach outperforms the class-balanced weighting scheme for both the cross-entropy loss and the focal loss, as we observed in the main paper. Moreover, our results are on par with best reported ones except on ImageNet-LT. Finally, we stress that almost all existing methods employ a class-balanced weighting or sampling strategy no matter what their main techniques are to tackle the long-tailed problem. Hence, given our consistent improvements over the class-balanced weighting, we expect the methods which have benefited from the class-balancing can gain further from our two-component weighting.


% %%%%%%% ImageNet-LT Table%%%%%%%%%%


% \begin{table*}[h!]
% \centering
% \caption {\label{tab:ImageNet-LT} Test top-1 errors (\%) of different methods on ImageNet-LT. * indicates the re-run results.}
% \vspace{2pt}
% \resizebox{1.0\textwidth}{!}{%
% \begin{tabular}{l|l|l|l|l|l|l|l}
% \hline

% \hline

% \hline
% Methods & \multicolumn{1}{c|}{NN} & Initialization & Sampling & Loss & \begin{tabular}[c]{@{}l@{}}Stage-1\\ Trainable Variables\end{tabular} & \begin{tabular}[c]{@{}l@{}}Stage-2\\ Trainable Variables\end{tabular} & Results \\ \hline

% Vanilla Model & ResNet-10 & No-pretrain & Class-Balanced &  CE & All  & - & 80.0 \\ \hline

% Vanilla Model~\cite{Focalloss} & ResNet-10 &No-pretrain  & Class-Balanced & Focal &All   &-  & 69.8 \\ \hline


% Vanilla Model & ResNet-10 & No-pretrain  &Class-Balanced  &  Lifted&All  &-  & 69.2 \\ \hline

% Vanilla Model~\cite{Rangeloss} & ResNet-10 & No-pretrain & Class-Balanced &  Range & All & - & 69.3 \\ \hline

% Joint~\cite{kang2019decoupling} &ResNet-10  & No-pretrain &Class-Balanced  & CE & All & All & 65.2 \\ \hline

% NCM~\cite{kang2019decoupling} & ResNet-10 & No-pretrain &Class-Balanced  & CE &All  & Classifier layer & 64.5  \\ \hline

% cRT~\cite{kang2019decoupling} & ResNet-10 & No-pretrain &Class-Balanced  &CE  &All  &  Classifier layer& \textbf{58.2} \\ \hline

% $\tau$-normalized~\cite{kang2019decoupling} & ResNet-10 & No-pretrain &Class-Balanced  &  CE&All  &Classifier layer  & \underline{59.4}    \\ \hline

% OLTR*~\cite{OLTR} & ResNet-10  & No-pretrain &Class-Balanced  &CE  &All  & All & 65.6  \\ \hline

% OLTR~\cite{OLTR} & ResNet-10 & No-pretrain &Class-Balanced  &CE  &All  & All & 64.4 \\ \hline

% Ours & ResNet-10 & No-pretrain & None  &CE  & All & Classifier layer & 63.5 \\ \hline

% Ours & ResNet-10  & No-pretrain & None & Focal &All  &Classifier layer  & 63.3 \\ \hline

% \hline

% \hline

% Vanilla Model & ResNet-50  & No-pretrain & None & CE & All  & -  & 59.0 \\ \hline

% CB~\cite{CBLoss} & ResNet-50 & No-pretrain & None &  CE& All & - & 58.2 \\ \hline
% Joint~\cite{kang2019decoupling} &ResNet-50  & No-pretrain &Class-Balanced  & CE & All & All & 58.4 \\ \hline

% NCM~\cite{kang2019decoupling} & ResNet-50 & No-pretrain &Class-Balanced  & CE &All  & Classifier layer & 55.7  \\ \hline

% cRT~\cite{kang2019decoupling} & ResNet-50 & No-pretrain &Class-Balanced  &CE  &All  &  Classifier layer& \underline{52.7} \\ \hline

% $\tau$-normalized~\cite{kang2019decoupling} & ResNet-50 & No-pretrain &Class-Balanced  &  CE&All  &Classifier layer  & 53.3   \\ \hline

% Ours & ResNet-50  & No-pretrain & None & CE &All  &Classifier layer  &  \textbf{52.0} \\ \hline

% \end{tabular}
% }%
% \end{table*}






% %%%%%%% Places-LT Table%%%%%%%%%%


% \begin{table*}[h!]
% \centering
% \caption {\label{tab:Places-LT} Test top-1 errors (\%) of different methods on Places-LT. * indicates the re-run results.}
% \vspace{2pt}
% \resizebox{1.0\textwidth}{!}{%
% \begin{tabular}{l|l|l|l|l|l|l|l}
% \hline

% \hline

% \hline
% Methods & \multicolumn{1}{c|}{NN} & Initialization & Sampling & Loss & \begin{tabular}[c]{@{}l@{}}Stage-1\\ Trainable Variables\end{tabular} & \begin{tabular}[c]{@{}l@{}}Stage-2\\ Trainable Variables\end{tabular} & Results \\ \hline
% Vanilla Model & ResNet-152  & ImageNet & Class-Balanced  & CE & \begin{tabular}[c]{@{}l@{}} FC layers\\ Last Block + FC\end{tabular} & \begin{tabular}[c]{@{}l@{}}-\\ -\end{tabular} & \begin{tabular}[c]{@{}l@{}} 72.1\\ 69.7\end{tabular} \\ \hline
% Vanilla Model~\cite{Focalloss} & ResNet-152  & ImageNet & Class-Balanced  & Focal & \begin{tabular}[c]{@{}l@{}} FC layers\\ Last Block + FC\end{tabular} & \begin{tabular}[c]{@{}l@{}}-\\ -\end{tabular} & \begin{tabular}[c]{@{}l@{}}67.0\\ 66.5\end{tabular} \\ \hline
% Vanilla Model & ResNet-152  & ImageNet & Class-Balanced & Lifted & FC layers & - & 64.8 \\ \hline
% Vanilla Model~\cite{Rangeloss} & ResNet-152 &ImageNet  &Class-Balanced  & Range&  FC layers & - & 64.9 \\ \hline

% Joint~\cite{kang2019decoupling} & ResNet-152  &ImageNet  & Class-Balanced & CE & Last block + FC & Last block + FC & 69.8 \\ \hline

% NCM~\cite{kang2019decoupling} &ResNet-152  &ImageNet  &Class-Balanced  & CE & Last block + FC  & Classifier layer & 63.7 \\ \hline

% cRT~\cite{kang2019decoupling} &ResNet-152  &ImageNet  & Class-Balanced &CE  &Last block + FC  &Classifier layer  & 63.3 \\ \hline

% $\tau$-normalized~\cite{kang2019decoupling} & ResNet-152 & ImageNet &Class-Balanced  & CE &Last block + FC  & Classifier layer  &\textbf{62.1}  \\ \hline

% OLTR*~\cite{OLTR} &ResNet-152  &ImageNet  & Class-Balanced &CE  &Last block + FC  & FC + memory  & 64.8 \\ \hline

% OLTR~\cite{OLTR} & ResNet-152 &ImageNet  &Class-Balanced  & CE & Last block + FC & FC + memory & 64.1 \\ \hline

% Ours &ResNet-152  &ImageNet  & None  & CE &Last block + FC  & Classifier layer & 62.9 \\ \hline

% Ours & ResNet-152 &ImageNet  & None & Focal &Last block + FC  & Classifier layer & \underline{62.2} \\ \hline


% \end{tabular}
% }%
% \end{table*}


% %%%%%%% iNat Table%%%%%%%%%%



% \begin{table*}[h!]
% \centering
% \caption {\label{tab:iNat18} Test top-1 errors (\%) of different methods on iNaturalist 2018.}
% \vspace{2pt}
% \resizebox{1.0\textwidth}{!}{%

% \begin{tabular}{l|l|l|l|l|l|l|l}
% \hline

% \hline

% \hline
% Methods & \multicolumn{1}{c|}{NN} & Initialization & Sampling & Loss & \begin{tabular}[c]{@{}l@{}}Stage-1\\ Trainable Variables\end{tabular} & \begin{tabular}[c]{@{}l@{}}Stage-2\\ Trainable Variables\end{tabular} & Results \\ \hline


% Vanilla Model & ResNet-50 & No-pretrain & None & CE & All & -& 42.9 \\ \hline
% Vanilla Model & ResNet-50  & ImageNet+iNat'17  & None  & CE  & All & - & 36.2 \\ \hline

% LDAM~\cite{LDAM} & ResNet-50 & No-pretrain  & None & LDAM & All & - & 35.4 \\ \hline
% LDAM-DRW~\cite{LDAM} & ResNet-50  & No-pretrain  & None & LDAM & All &-  & \textbf{32.0} \\ \hline


% CB~\cite{CBLoss} & ResNet-50 & ImageNet+iNat'17 & None &  CE& All & - & 34.7 \\ \hline
% CB~\cite{CBLoss} & ResNet-50 & No-pretrain &None  &Focal  & All & - & 38.9 \\ \hline

% Joint~\cite{kang2019decoupling} & ResNet-50 &No-pretrain  &Class-Balanced  & CE & All & All  & 38.3 \\ \hline

% NCM~\cite{kang2019decoupling} &ResNet-50  & No-pretrain & Class-Balanced &CE  &All  & Classifier layer  & 41.8 \\ \hline

% cRT~\cite{kang2019decoupling} &ResNet-50  & No-pretrain &Class-Balanced  & CE & All & Classifier layer & 34.8 \\ \hline

% $\tau$-normalized~\cite{kang2019decoupling} &ResNet-50  & No-pretrain & Class-Balanced & CE & All & Classifier layer & 34.4 \\ \hline

% Ours &ResNet-50  & ImageNet+iNat'17 & None &CE  & All & All & \underline{32.4} \\ \hline

% Ours &ResNet-50  & ImageNet+iNat'17 & None &Focal  & All & All & \underline{32.3} \\ \hline

% \hline

% \hline


% Vanilla Model & ResNet-101  & ImageNet+iNat'17  & None  & CE  & All & - & 34.3 \\ \hline

% CB~\cite{CBLoss} & ResNet-101  & ImageNet+iNat'17  & None  & CE  & All & - & 32.7 \\ \hline

% Ours &ResNet-101  & ImageNet+iNat'17 & None & CE  & All & All & \textbf{31.5} \\ \hline
% \end{tabular}
% }%
% \end{table*}





% % \begin{table}[h!]
% % \caption {\label{tab:inat-resnet101} Classification error rates \% on iNaturalist 2018 using ResNet-101 (To be removed).}
% % \vspace{5pt}
% % \resizebox{1.0\linewidth}{!}{%

% % \begin{tabular}{l|c|l|l}
% % \hline
% % Dataset Name & \multicolumn{3}{c}{iNat2018} \\ \hline
% % Methods & Top-1 & Top-3 & Top-5 \\ \hline
% % Cross-Entropy Loss & 34.26 & 19.37  & 15.04 \\ \hline
% % Class-Balance Loss~\cite{CBLoss} & 32.66  & 18.58 & 14.97 \\ \hline
% % Ours & \textbf{31.53} & \textbf{17.25}  & \textbf{13.16} \\ \hline

% % \end{tabular}
% % }%

% % \end{table}










% {\small
% \bibliographystyle{ieee_fullname}
% \bibliography{references}
% }


% \end{document}
